# Supplementary material for: Signatures of the Correlated-Hopping Interaction in Non-Linear Transport through a Quantum Dot
Source: arXiv:2411.19850 ancillary file (2024-11-29)
Supplement: Supplementary file 1 [file nonlinear2024_SM.pdf]

# Supplemental Material: Signatures of the Correlated-Hopping Interaction in Non-Linear Transport through a Quantum Dot


Ulrich Eckern
*Institute of Physics, University of Augsburg,*
*86135 Augsburg, Germany*
*ulrich.eckern@physik.uni-augsburg.de*
*https://orcid.org/0000-0001-8917-9083*

Karol I. Wysokiński
*Institute of Physics, M. Curie-Skłodowska University,*
*pl. M. Curie-Skłodowskiej 1, 20-031 Lublin, Poland*
*karol.wysokinski@umcs.lublin.pl*
*https://orcid.org/0000-0002-5366-4455*



We rewrite here the final formulae for the transport and spectral Green functions. The details of calculations of the lifetimes up to second order in the couplings $\Gamma_\sigma^\lambda$, i.e., up to fourth order in the tunneling amplitudes $V_{\lambda k\sigma}$, are presented.


## I. GREEN FUNCTIONS

Here we reiterate the final expressions for the two Green functions calculated earlier [1].

### A. Transport Green function

The transport GF $\langle\langle D_\sigma|D_\sigma^\dagger\rangle\rangle_\omega$ reads

$$\langle\langle D_\sigma|D_\sigma^\dagger\rangle\rangle_\omega = \frac{1-x(2-x)(\langle n_{\bar\sigma}\rangle + \tilde b_{1\bar\sigma}) + n_{\rm eff}^D(\omega) I_D(\omega)}{\omega - \varepsilon_d - \Sigma_{0\sigma} + \Sigma_D(\omega)}, \tag{1}$$

where

$$I_D(\omega) = \frac{U - x(2-x)(\Sigma_{0\sigma} + \Sigma_{\bar\sigma}^{(1)})}{\omega - \varepsilon_\sigma - U - \Sigma_{ID}(\omega)}, \tag{2}$$

and

$$\begin{aligned} n_{\rm eff}^D(\omega) &= (1-x)^2(\langle n_{\bar\sigma}\rangle + \tilde b_{1\bar\sigma}) - \bar b_{2\bar\sigma}, & (3)\\ B_D(\omega) &= (1-x)^2[\tilde b_{1\bar\sigma}\Sigma_{0\sigma} - \Sigma_{1\bar\sigma}^T - \Sigma_{2\bar\sigma}^T] - \bar b_{2\bar\sigma}\Sigma_{0\sigma}, & (4)\\ \Sigma_D(\omega) &= x(2-x)(\tilde b_{1\bar\sigma}\Sigma_{0\sigma} - \Sigma_{1\bar\sigma}^T) - I_D(\omega)B_D(\omega), & (5)\\ \Sigma_{ID}(\omega) &= (1-x)^2(\Sigma_{0\sigma} + \Sigma_{\bar\sigma}^{(1)}) - x(2-x)\Sigma_{2\bar\sigma}^T + \Sigma_{\bar\sigma}^{(2)}. & (6) \end{aligned}$$

For various definitions and details, see [1].

### B. Spectral Green function

The spectral GF $\langle\langle d_\sigma|d_\sigma^\dagger\rangle\rangle_\omega$ is found as

$$\langle\langle d_\sigma|d_\sigma^\dagger\rangle\rangle_\omega = \frac{1 - x(\tilde b_{1\bar\sigma} + \tilde b_{2\bar\sigma}) + n_{\rm eff}^d(\omega) I_d(\omega)}{\omega - \varepsilon_d - \Sigma_{0\sigma} + x[(\tilde b_{1\bar\sigma} + \tilde b_{2\bar\sigma})\Sigma_{0\sigma} - \Sigma_{1\bar\sigma}^T + (1-x)\Sigma_{2\bar\sigma}^T] - I_d(\omega)B_d(\omega)}, \tag{7}$$

where

$$I_d(\omega) = \frac{U - x(2-x)\Sigma_{0\sigma} + x(1-x)\Sigma^{(1)}_{\bar\sigma} - x\Sigma^{(2)}_{\bar\sigma} - x^2[\Sigma^T_{1\bar\sigma} + \Sigma^T_{2\bar\sigma} - (\tilde b_{1\bar\sigma} + \tilde b_{2\bar\sigma})\Sigma_{0\sigma}]}{\omega - \varepsilon_\sigma - U - (1-x)^2(\Sigma_{0\sigma} + \Sigma^{(1)}_{\bar\sigma}) - \Sigma^{(2)}_{\bar\sigma} - x(\tilde b_{2\bar\sigma}\Sigma_{0\sigma} - \Sigma^T_{2\bar\sigma}) + x(1-x)(\tilde b_{1\bar\sigma}\Sigma_{0\sigma} - \Sigma^T_{1\bar\sigma})}, \tag{8}$$

and

$$n^d_{\text{eff}}(\omega) = \langle n_{\bar\sigma}\rangle + (1-x)\tilde b_{1\sigma} - \bar b_{2\sigma} \tag{9}$$

$$B_d(\omega) = [(1-x)\tilde b_{1\bar\sigma} - \bar b_{2\bar\sigma}]\Sigma_{0\sigma} - (1-x)(\Sigma^T_{1\bar\sigma} + \Sigma^T_{2\bar\sigma}). \tag{10}$$

It has to be stressed that both GFs, *i.e.*, the spectral and transport GFs, are coupled together. They have to be calculated simultaneously as various quantities they depend on require the knowledge of both of them.

All parameters are defined in [1], and we quote here some of them, together with the definions in terms of various Green functions.

$$\tilde b_{1\bar\sigma}(\omega) = \sum_{\lambda k} \frac{V^*_{\lambda k\bar\sigma}\langle D^\dagger_{\bar\sigma} c_{\lambda k\bar\sigma}\rangle}{\omega - \varepsilon_{\lambda k} - \varepsilon_1 + i\tilde\gamma^{\bar\sigma}_1}$$
$$= \int \frac{d\varepsilon}{2\pi} \frac{\sum_\lambda \Gamma^\lambda_{\bar\sigma} f_\lambda(\varepsilon)\langle\langle D_{\bar\sigma}|D^\dagger_{\bar\sigma}\rangle\rangle^a_\varepsilon}{\omega - \varepsilon - \varepsilon_1 + i\tilde\gamma^{\bar\sigma}_1}. \tag{11}$$

$$b_{2\bar\sigma}(\omega) = \sum_{\lambda k} \frac{V_{\lambda k\bar\sigma}\langle c^\dagger_{\lambda k\bar\sigma} d_{\bar\sigma}\rangle}{\omega + \varepsilon_{\lambda k} - \varepsilon_2 + i\tilde\gamma_2}$$
$$= \int \frac{d\varepsilon}{2\pi} \frac{\sum_\lambda \Gamma^\lambda_{\bar\sigma} f_\lambda(\varepsilon)\langle\langle d_{\bar\sigma}|D^\dagger_{\bar\sigma}\rangle\rangle^r_\varepsilon}{\omega + \varepsilon - \varepsilon_2 + i\tilde\gamma_2}, \tag{12}$$

and

$$N_{2\bar\sigma}(\omega) = \sum_{\lambda k} \frac{V_{\lambda k\bar\sigma}\langle c^\dagger_{\lambda k\bar\sigma} d_{\bar\sigma} n_{\bar\sigma}\rangle}{\omega + \varepsilon_{\lambda k} - \varepsilon_2 + i\tilde\gamma_2}$$
$$= \int \frac{d\varepsilon}{2\pi} \frac{\sum_\lambda \Gamma^\lambda_{\bar\sigma} f_\lambda(\varepsilon)\langle\langle n_\sigma d_{\bar\sigma}|D^\dagger_{\bar\sigma}\rangle\rangle^r_\varepsilon}{\omega + \varepsilon - \varepsilon_2 + i\tilde\gamma_2} \tag{13}$$

$$\bar b_{2\bar\sigma}(\omega) = (1-x)^2 \int \frac{d\varepsilon}{2\pi} \frac{\sum_\lambda \Gamma^\lambda_{\bar\sigma} f_\lambda(\varepsilon)\langle\langle D_{\bar\sigma}|D^\dagger_{\bar\sigma}\rangle\rangle^r_\varepsilon}{\omega + \varepsilon - \varepsilon_2 + i\tilde\gamma_2}$$
$$+x(2-x) \int \frac{d\varepsilon}{2\pi} \frac{\sum_\lambda \Gamma^\lambda_{\bar\sigma} f_\lambda(\varepsilon)\langle\langle n_\sigma D_{\bar\sigma}|D^\dagger_{\bar\sigma}\rangle\rangle^r_\varepsilon}{\omega + \varepsilon - \varepsilon_2 + i\tilde\gamma_2}. \tag{14}$$

$$\Sigma^T_{1\bar\sigma}(\omega) = \sum_{\lambda k}\sum_{\lambda' k'} \frac{V^*_{\lambda k\bar\sigma} V_{\lambda' k'\bar\sigma}\langle c^\dagger_{\lambda' k'\bar\sigma} c_{\lambda k\bar\sigma}\rangle}{\omega - \varepsilon_{\lambda k} - \varepsilon_1 + i\tilde\gamma^{\bar\sigma}_1}$$
$$= \int \frac{d\varepsilon}{2\pi} \frac{\sum_\lambda \Gamma^\lambda_{\bar\sigma} f_\lambda(\varepsilon)[1 + \frac{i}{2}\Gamma_{\bar\sigma}\langle\langle D_{\bar\sigma}|D^\dagger_{\bar\sigma}\rangle\rangle^a_\varepsilon]}{\omega - \varepsilon - \varepsilon_1 + i\tilde\gamma^{\bar\sigma}_1} \tag{15}$$

$$\Sigma^T_{2\bar\sigma}(\omega) = \sum_{\lambda k}\sum_{\lambda' k'} \frac{V_{\lambda k\bar\sigma} V^*_{\lambda' k'\bar\sigma}\langle c^\dagger_{\lambda k\bar\sigma} c_{\lambda' k'\bar\sigma}\rangle}{\omega + \varepsilon_{\lambda k} - \varepsilon_2 + i\tilde\gamma_2}$$
$$= \int \frac{d\varepsilon}{2\pi} \frac{\sum_\lambda \Gamma^\lambda_{\bar\sigma} f_\lambda(\varepsilon)[1 - \frac{i}{2}\Gamma_{\bar\sigma}\langle\langle D_{\bar\sigma}|D^\dagger_{\bar\sigma}\rangle\rangle^r_\varepsilon]}{\omega + \varepsilon - \varepsilon_2 + i\tilde\gamma_2} \tag{16}$$

The following self-energies:

$$\Sigma^{(1)}_{\bar\sigma} = \sum_{\lambda k} \frac{|V_{\lambda k\bar\sigma}|^2}{\omega - \varepsilon_{\lambda k} - \varepsilon_1 + i\tilde\gamma^{\bar\sigma}_1}, \tag{17}$$

$$\Sigma^{(2)}_{\bar\sigma} = \sum_{\lambda k} \frac{|V_{\lambda k\bar\sigma}|^2}{\omega + \varepsilon_{\lambda k} - \varepsilon_2 + i\tilde\gamma_2}, \tag{18}$$

are evaluated with appropriate lifetimes calculated below. The inverse lifetimes in the above formulae are sums of second and fourth order contributions discussed in the next section. We recall that

$$\tilde\gamma^\sigma_1 = \gamma^{(2)}_\sigma + \gamma^{(4)}_\sigma, \tag{19}$$

$$\tilde\gamma_2 = \gamma^{(2)}_D + \gamma^{(4)}_D. \tag{20}$$

In addition, the energies $\varepsilon_{1(2)}$ are defined as

$$\varepsilon_1 = \varepsilon_\sigma - \varepsilon_{\bar\sigma}, \tag{21}$$

$$\varepsilon_2 = \varepsilon_\sigma + \varepsilon_{\bar\sigma} + U. \tag{22}$$

## II. LIFETIMES: SECOND AND FOURTH ORDER CONTRIBUTIONS

The excited states of the system are subject to emission processes which determine their respective lifetimes. Lifetime effects [2, 3] are of primary importance in the non-linear regime. The decay rates (inverse lifetimes) can be estimated using Fermi's golden rule. The complication arising in non-equilibrium situations is that they have to be calculated up to fourth order with all possible intermediate and final states taken into account.

The quantum dot maybe singly or doubly occupied with the Fock states $|i_\sigma\rangle \propto d^\dagger_\sigma$ or $|i_D\rangle \propto d^\dagger_\sigma d^\dagger_{\bar\sigma}$ respectively. Fermi's golden rule up to *second order* in the coupling reads

$$\gamma^{(2)}_i = 2\pi \sum_f |\langle f|H_T|i\rangle|^2 \delta(E_i - E_f), \tag{23}$$

where $H_T = \sum_{\lambda k\sigma}\left(V_{\lambda k\sigma} c^\dagger_{\lambda k\sigma} D_\sigma + V^*_{\lambda k\sigma} D^\dagger_\sigma c_{\lambda k\sigma}\right)$ is the tunnelling part of the Hamiltonian, $|i\rangle$, $E_i$ ($|f\rangle, E_f$) denote the initial (final) state and its energy. With correlated hopping taken into account, one finds the following expressions valid to second order in the dot coupling

$V_{\lambda k\sigma}$:

$$\gamma_\sigma^{(2)} = \sum_\lambda \left(\Gamma_\sigma^\lambda[1-f_\lambda(\varepsilon_\sigma)] + (1-x)^2\Gamma_{\bar\sigma}^\lambda f_\lambda(\varepsilon_{\bar\sigma}+U)\right),$$
$$\gamma_D^{(2)} = (1-x)^2\sum_{\lambda\sigma}\Gamma_\sigma^\lambda[1-f_\lambda(\varepsilon_\sigma+U)]. \quad (24)$$

Importantly, the lifetimes do depend on the ratio $x$ between the interaction induced and direct couplings between the dot and the electrodes. The second expression shows that the contribution from the doubly occupied state vanishes for $x=1$, as expected. For this value of $x$ the doubly occupied state is totally decoupled from the system.

In the *fourth order* in the coupling, the lifetimes are calculated as

$$\gamma_i^{(4)} = 2\pi\sum_f\left|\sum_n\langle f|H_T|n\rangle\frac{1}{E_i-E_n}\langle n|H_T|i\rangle\right|^2\delta(E_i-E_f)$$
$$= 2\pi\sum_{f,n,m}\langle f|H_T|n\rangle\frac{1}{E_i-E_n}\langle n|H_T|i\rangle\times \quad (25)$$
$$\times\ \langle i|H_T|m\rangle\frac{1}{E_i-E_m}\langle m|H_T|f\rangle\delta(E_i-E_f),$$

where $|n\rangle,|m\rangle$ are intermediate states with energies $E_n$ and $E_m$. Introducing $H_T$ into the last equation one gets six terms which contribute, in principle at least, to the lifetimes. They read:

$$I_1 = V_{\lambda'k'\sigma'}V_{\lambda k\sigma}V^*_{\lambda''k''\sigma''}V^*_{\lambda_3k_3\sigma_3}\langle f|c^\dagger_{\lambda'k'\sigma'}D_{\sigma'}|n\rangle \quad (26)$$
$$\times\ \langle n|c^\dagger_{\lambda k\sigma}D_\sigma|i\rangle\cdot\langle i|D^\dagger_{\sigma''}c_{\lambda''k''\sigma''}|m\rangle\langle m|D^\dagger_{\sigma_3}c_{\lambda_3k_3\sigma_3}|f\rangle$$
$$I_2 = V^*_{\lambda'k'\sigma'}V_{\lambda k\sigma}V_{\lambda''k''\sigma''}V^*_{\lambda_3k_3\sigma_3}\langle f|D^\dagger_{\sigma'}c_{\lambda'k'\sigma'}|n\rangle \quad (27)$$
$$\times\ \langle n|c^\dagger_{\lambda k\sigma}D_\sigma|i\rangle\cdot\langle i|c^\dagger_{\lambda''k''\sigma''}D_{\sigma''}|m\rangle\langle m|D^\dagger_{\sigma_3}c_{\lambda_3k_3\sigma_3}|f\rangle$$
$$I_3 = V^*_{\lambda'k'\sigma'}V_{\lambda k\sigma}V^*_{\lambda''k''\sigma''}V_{\lambda_3k_3\sigma_3}\langle f|D^\dagger_{\sigma'}c_{\lambda'k'\sigma'}|n\rangle \quad (28)$$
$$\times\ \langle n|c^\dagger_{\lambda k\sigma}D_\sigma|i\rangle\cdot\langle i|D^\dagger_{\sigma''}c_{\lambda''k''\sigma''}|m\rangle\langle m|c^\dagger_{\lambda_3k_3\sigma_3}D_{\sigma_3}|f\rangle$$
$$I_4 = V_{\lambda'k'\sigma'}V^*_{\lambda k\sigma}V_{\lambda''k''\sigma''}V^*_{\lambda_3k_3\sigma_3}\langle f|c^\dagger_{\lambda'k'\sigma'}D_{\sigma'}|n\rangle \quad (29)$$
$$\times\ \langle n|D^\dagger_\sigma c_{\lambda k\sigma}|i\rangle\cdot\langle i|c^\dagger_{\lambda''k''\sigma''}D_{\sigma''}|m\rangle\langle m|D^\dagger_{\sigma_3}c_{\lambda_3k_3\sigma_3}|f\rangle$$
$$I_5 = V_{\lambda'k'\sigma'}V^*_{\lambda k\sigma}V^*_{\lambda''k''\sigma''}V_{\lambda_3k_3\sigma_3}\langle f|c^\dagger_{\lambda'k'\sigma'}D_{\sigma'}|n\rangle \quad (30)$$
$$\times\ \langle n|D^\dagger_\sigma c_{\lambda k\sigma}|i\rangle\cdot\langle i|D^\dagger_{\sigma''}c_{\lambda''k''\sigma''}|m\rangle\langle m|c^\dagger_{\lambda_3k_3\sigma_3}D_{\sigma_3}|f\rangle$$
$$I_6 = V^*_{\lambda'k'\sigma'}V^*_{\lambda k\sigma}V_{\lambda''k''\sigma''}V_{\lambda_3k_3\sigma_3}\langle f|D^\dagger_{\sigma'}c_{\lambda'k'\sigma'}|n\rangle \quad (31)$$
$$\times\ \langle n|D^\dagger_\sigma c_{\lambda k\sigma}|i\rangle\cdot\langle i|c^\dagger_{\lambda''k''\sigma''}D_{\sigma''}|m\rangle\langle m|c^\dagger_{\lambda_3k_3\sigma_3}D_{\sigma_3}|f\rangle$$

**Doubly occupied dot**

For the doubly occupied state on the dot, one starts with $|i_D^\dagger\rangle$ given above, and finds the following intermediate states connected by the tunnelling part of the Hamiltonian:

$$|n_\sigma\rangle \propto c^\dagger_{\lambda k\sigma}d^\dagger_{\bar\sigma} \quad (32)$$

for both directions of the spin, to be summed over. The two possible final states are obtained either by annihilating the state on the dot and creating an appropriate one in one of the electrodes:

$$|f\rangle \propto c^\dagger_{\lambda'k'\bar\sigma}c^\dagger_{\lambda k\sigma}|0\rangle, \quad (33)$$

or by creating a second electron on the dot and simultaneously annihilating one with the same spin at the electrode. The last process results in

$$|f'\rangle \propto c_{\lambda'k'\sigma}c^\dagger_{\lambda k\sigma}d^\dagger_\sigma d^\dagger_{\bar\sigma}. \quad (34)$$

In the next step we calculate the energies of all involved states. With $E_0$ denoting the ground state energy of the electrons in the electrodes one finds

$$E_{i_D} = E_0+\varepsilon_\sigma+\varepsilon_{\bar\sigma}+U, \quad (35)$$

$$E_n = E_0+\varepsilon_{\lambda k\sigma}+\varepsilon_{\bar\sigma}, \quad (36)$$

$$E_f = E_0+\varepsilon_{\lambda k\sigma}+\varepsilon_{\lambda'k'\bar\sigma}, \quad (37)$$

and

$$E_{f'} = E_0+\varepsilon_\sigma+\varepsilon_{\bar\sigma}+U+\varepsilon_{\lambda k\sigma}-\varepsilon_{\lambda'k'\bar\sigma}. \quad (38)$$

We find that for the doubly occupied state on the dot, indicated by the subscript $D$, most of the terms in Eqs. (26–31) vanish, and only the terms $I_1$ and $I_6$ give non-vanishing contributions which sum up to the final result

$$\gamma_D^{(4)} = \frac{(1-x)^2}{2\pi}\sum_{\lambda,\lambda',\sigma}\int d\varepsilon\frac{1-f_\lambda(\varepsilon)}{(\varepsilon-\varepsilon_\sigma-U)^2}\Big[(1-x)^2\Gamma_\sigma^\lambda\Gamma_\sigma^{\lambda'}\times$$
$$\times\ f_{\lambda'}(\varepsilon)+\Gamma_\sigma^\lambda\Gamma_{\bar\sigma}^{\lambda'}[1-f_{\lambda'}(\varepsilon_\sigma+\varepsilon_{\bar\sigma}+U-\varepsilon)]\Big]. \quad (39)$$

It has to be noted that for $x=0$ our result slightly differs from that reported by Lavagna [2]: We find that the spins $\sigma$ and $\bar\sigma$ enter the couplings $\Gamma^\lambda$ and $\Gamma^{\lambda'}$ in the second term in the opposite order.

**Singly occupied dot**

A similar analysis for the lifetime of the singly occupied dot with

$$|i_\sigma\rangle \propto d^\dagger_\sigma \quad (40)$$

leads to two different intermediate states:

$$|n_1\rangle \propto c^\dagger_{\lambda k\sigma} \quad (41)$$

and

$$|n_2\rangle \propto c_{\lambda k\bar\sigma}d^\dagger_\sigma d^\dagger_{\bar\sigma}. \quad (42)$$

These states, in turn, result in four possible final states, which are of the following form:

$$
\begin{aligned}
|f_1\rangle &\propto c_{\lambda' k' \sigma} c^\dagger_{\lambda k \sigma} d^\dagger_\sigma, && (43)\\
|f_2\rangle &\propto c_{\lambda' k' \bar\sigma} c^\dagger_{\lambda k \sigma} d^\dagger_{\bar\sigma}, && (44)\\
|f_3\rangle &\propto c^\dagger_{\lambda' k' \bar\sigma} c_{\lambda k \bar\sigma} d^\dagger_\sigma, && (45)\\
|f_4\rangle &\propto c^\dagger_{\lambda' k' \sigma} c_{\lambda k \bar\sigma} d^\dagger_{\bar\sigma}. && (46)
\end{aligned}
$$

We shall need the energies of all the above states to evaluate (25). We also have to analyse the appropriate contributions from each of the terms $I_i$.

$I_1$: As an example, let us consider in detail two of them for the singly occupied dot with $|i\rangle = |i_\sigma\rangle$, starting with $I_1$. A non-zero value of the matrix element $\langle n|c^\dagger_{\lambda k\sigma} D_\sigma|i_\sigma\rangle$ requires the state $|n\rangle$ to not contain any spin on the dot. However, the matrix element to the left of the above one, namely $\langle f|c^\dagger_{\lambda' k'\sigma'} D_{\sigma'}|n\rangle$, vanishes if the dot is not occupied by an electron. Thus the contribution of this term to the lifetime vanishes, $I_1 = 0$.

$I_2$: To find the contribution to the lifetime of the considered state stemming from the term $I_2$, we start again with the matrix element with the known initial state, which now reads $\langle n|c^\dagger_{\lambda k\sigma} D_\sigma|i\rangle$. For $|i\rangle = |i_\sigma\rangle$ one notes that it can be written as $\langle n|c^\dagger_{\lambda k\sigma} d_\sigma|i_\sigma\rangle$, and the state $|n\rangle$ is again found to not have any electron on the dot. However, it has to have the state $\lambda k\sigma$ occupied and is thus the state denoted by $|n_1\rangle$. The matrix element to the left of the considered, $\langle f|D^\dagger_{\sigma'} c_{\lambda' k'\sigma'}|n\rangle$, does not constrain the value of the spin $\sigma'$, which at this stage remains arbitrary ($\sigma$ or $\bar\sigma$). The other matrix element of interest is that between initial (known) state and state $|m\rangle$. It reads $\langle i|c^\dagger_{\lambda'' k''\sigma''} D_{\sigma''}|m\rangle$, and we know that the left hand side state is $\langle i_\sigma|$, i.e., the state with a spin $\sigma$ electron on the dot. The operator $D_{\sigma''}$ annihilates a state with spin $\sigma''$. However, this cannot be the spin $\sigma$: for the matrix element to have a non-vanishing value, it is rather required that $\sigma'' = \bar\sigma$. Thus $|m\rangle$ has two electrons on the dot and no electron in the leads' state $\lambda'' k''\bar\sigma$. The action of the operator $D_{\sigma''} = D_{\bar\sigma}$ on $|m\rangle$ hence gives $(1-x)d_{\bar\sigma}|m\rangle$. Again we note that $\sigma_3$ is not constraint, but we can conclude that the final state $|f\rangle$ has the dot state with spin $\bar\sigma_3$ to be occupied. This in turn implies that the action of the operator $D^\dagger_{\sigma_3}$ produces another factor $(1-x)$. We still need to identify which spins $\sigma'$ and $\sigma_3$ will contribute, and which of the possible final states is realised. To this end, it is convenient to rewrite the adequate term as

$$
\begin{aligned}
I_2 &= V^*_{\lambda' k'\sigma'} V_{\lambda k\sigma} V_{\lambda'' k''\bar\sigma} V^*_{\lambda_3 k_3\sigma_3} (1-x)^2 \\
&\times \langle i|c^\dagger_{\lambda'' k''\bar\sigma} d_{\bar\sigma}|m\rangle\langle m|d^\dagger_{\sigma_3} c_{\lambda_3 k_3\sigma_3}|f\rangle \qquad (47)\\
&\times \langle f|d^\dagger_{\sigma'} c_{\lambda' k'\sigma'}|n\rangle\langle n|c^\dagger_{\lambda k\sigma} d_\sigma|i\rangle.
\end{aligned}
$$

The uniqueness of the final state constrains both arbitrary spins, hence $\sigma' = \bar\sigma$, $\sigma_3 = \sigma$, and we identify the final state with $|f_2\rangle$ given above. The opposite combination of spin signs is not allowed as can be easily checked.

Recalling that

$$
\begin{aligned}
E_i &= E_0 + \varepsilon_\sigma, && (48)\\
E_n &= E_{n_1} = E_0 + \varepsilon_{\lambda k\sigma}, && (49)\\
E_f &= E_0 + \varepsilon_{\bar\sigma} + \varepsilon_{\lambda k\sigma} - \varepsilon_{\lambda' k'\bar\sigma}, && (50)
\end{aligned}
$$

one finds this contribution to $\gamma^{(4)}_\sigma$ as

$$
\begin{aligned}
\gamma^{(4)}_\sigma(I_2) &= |V_{\lambda' k'\bar\sigma}|^2 |V_{\lambda k\sigma}|^2 (1-x)^2 \\
&\times \frac{\langle i|c^\dagger_{\lambda' k'\bar\sigma} c_{\lambda k\sigma} c_{\lambda' k'\bar\sigma} c^\dagger_{\lambda k\sigma}|i\rangle}{(\varepsilon_\sigma - \varepsilon_{\lambda k\sigma})(\varepsilon_{\lambda' k'\bar\sigma} - \varepsilon_{\bar\sigma} - U)} \qquad (51)\\
&\times \delta(\varepsilon_\sigma - \varepsilon_{\bar\sigma} - \varepsilon_{\lambda k\sigma} + \varepsilon_{\lambda' k'\bar\sigma}).
\end{aligned}
$$

Introducing into the last formula appropriate integrals over Dirac $\delta$-distributions, defining effective couplings

$$
\Gamma^\lambda_\sigma = 2\pi \sum_k |V_{\lambda k\sigma}|^2 \delta(\varepsilon - \varepsilon_{\lambda k\sigma}), \qquad (52)
$$

and averaging over all states corresponding to the initial one, we find

$$
\begin{aligned}
\gamma^{(4)}_\sigma(I_2) &= \frac{(1-x)^2}{2\pi} \int d\varepsilon \int d\varepsilon' \frac{[1-f_\lambda(\varepsilon)] f_{\lambda'}(\varepsilon')}{(\varepsilon_\sigma - \varepsilon)(\varepsilon' - \varepsilon_{\bar\sigma} - U)} \\
&\times \Gamma^{\lambda'}_{\bar\sigma} \Gamma^\lambda_\sigma \delta(\varepsilon_\sigma - \varepsilon_{\bar\sigma} - \varepsilon + \varepsilon'). \qquad (53)
\end{aligned}
$$

Integrating over $\varepsilon'$ leads to

$$
\gamma^{(4)}_\sigma(I_2) = \frac{(1-x)^2}{2\pi} \int d\varepsilon \frac{[1-f_\lambda(\varepsilon)] f_{\lambda'}(\varepsilon + \varepsilon_{\bar\sigma} - \varepsilon_\sigma) \Gamma^{\lambda'}_{\bar\sigma} \Gamma^\lambda_\sigma}{(\varepsilon - \varepsilon_\sigma)(\varepsilon - \varepsilon_\sigma - U)}. \qquad (54)
$$

$I_3$: All the remaining contributions to the lifetime of a singly occupied dot (the contribution from $I_6$ vanishes) are analysed in a similar way. For a singly occupied initial state the summation over $\sigma''$ in the term

$$
\begin{aligned}
I_3 &= V^*_{\lambda' k'\sigma'} V_{\lambda k\sigma} V^*_{\lambda'' k''\sigma''} V_{\lambda_3 k_3\sigma_3} \langle f|D^\dagger_{\sigma'} c_{\lambda' k'\sigma'}|n\rangle \qquad (55)\\
&\times \langle n|c^\dagger_{\lambda k\sigma} D_\sigma|i\rangle \cdot \langle i|D^\dagger_{\sigma''} c_{\lambda'' k''\sigma''}|m\rangle\langle m|c^\dagger_{\lambda_3 k_3\sigma_3} D_{\sigma_3}|f\rangle
\end{aligned}
$$

is restricted to $\sigma'' = \sigma$. Both states $|m\rangle$ and $|n\rangle$ are found to have no electron on the dot, thus reducing to $|n_1\rangle$ above. All operators $D_\sigma$, $D^\dagger_\sigma$ reduce to $d_\sigma$, $d^\dagger_\sigma$. The summations over $\sigma'$ and $\sigma_3$ are not restricted on this level. We note that two out of four possible combinations, namely $\sigma' = \sigma_3 = \sigma$ and $\sigma' = \sigma_3 = \bar\sigma$, lead to the two different (acceptable) final states $|f_1\rangle$ and $|f_2\rangle$. For both final states the summation over the remaining lead quantum numbers is restricted by the conditions $(\lambda'', k'') = (\lambda, k)$ and $(\lambda_3, k_3) = (\lambda', k')$. The $I_3$ term thus contributes

$$
\begin{aligned}
\gamma^{(4)}_\sigma(I_3) &= \frac{1}{2\pi} \sum_{\lambda,\lambda'} \int d\varepsilon \frac{[1-f_\lambda(\varepsilon)]}{(\varepsilon - \varepsilon_\sigma)^2} \qquad (56)\\
&\times \Big[\Gamma^\lambda_\sigma \Gamma^{\lambda'}_\sigma f_{\lambda'}(\varepsilon) + \Gamma^\lambda_\sigma \Gamma^{\lambda'}_{\bar\sigma} f_{\lambda'}(\varepsilon + \varepsilon_{\bar\sigma} - \varepsilon_\sigma)\Big].
\end{aligned}
$$

$I_4$: The contribution from $I_4$ is found similarly. The important difference is that one obtains a $(1-x)$ factor

from each term, the summation over $\sigma$ (the summation variable has not to be confused with fixed symbol for the initial state $|\sigma\rangle$) is restricted to $\sigma = \bar{\sigma}$, and summation over $\sigma''$ gives a non-vanishing contribution for $\sigma'' = \bar{\sigma}$. Again the remaining two summations over spin variables are not restricted. The intermediate states are both found to contain two electrons with opposite spins, i.e., they reduce to the $|n_2\rangle$ state. The unrestricted spins can take $\sigma$ values leading to the unique final state $|f_4\rangle$, or $\bar{\sigma}$ values and the final state $|f_3\rangle$. The final contribution related to $I_4$ reads

$$\gamma_\sigma^{(4)}(I_4) = \frac{(1-x)^4}{2\pi} \sum_{\lambda,\lambda'} \int d\varepsilon \frac{[1-f_\lambda(\varepsilon)]}{(\varepsilon - \varepsilon_\sigma - U)^2} \times \left[\Gamma_{\bar{\sigma}}^{\lambda} \Gamma_{\bar{\sigma}}^{\lambda'} f_{\lambda'}(\varepsilon) + \Gamma_{\sigma}^{\lambda} \Gamma_{\bar{\sigma}}^{\lambda'} f_{\lambda'}(\varepsilon + \varepsilon_{\bar{\sigma}} - \varepsilon_\sigma)\right]. \quad (57)$$

$I_5$: The last term which contributes to the lifetime of a singly occupied dot state is $I_5$ (as the $I_6$ part gives zero). Its detailed analysis is similar to $I_2$. The structure of operators close to the known initial state

$$I_5 = V_{\lambda' k' \sigma'} V^*_{\lambda k \sigma} V^*_{\lambda'' k'' \sigma''} V_{\lambda_3 k_3 \sigma_3} \langle f | c^\dagger_{\lambda' k' \sigma'} D_{\sigma'} | n \rangle \times \langle n | D^\dagger_{\sigma} c_{\lambda k \sigma} | i \rangle \cdot \langle i | D^\dagger_{\sigma''} c_{\lambda'' k'' \sigma''} | m \rangle \langle m | c^\dagger_{\lambda_3 k_3 \sigma_3} D_{\sigma_3} | f \rangle \quad (58)$$

suggests that the intermediate state $|n\rangle$ has to be the doubly occupied dot, while the intermediate state $|m\rangle$ is empty and thus $\sigma'' = \sigma$. Summation over $\sigma$ is reduced to $\bar{\sigma}$. The overall $x$ dependent factor is $(1-x)^2$, and the final state reduces to $|f_4\rangle$. Introducing all energies one finds the following contribution to $\gamma_\sigma^{(4)}$:

$$\gamma_\sigma^{(4)}(I_5) = |V_{\lambda' k' \sigma}|^2 |V_{\lambda k \bar{\sigma}}|^2 (1-x)^2 \times \frac{\langle i | c_{\lambda' k' \sigma} c^\dagger_{\lambda k \bar{\sigma}} c^\dagger_{\lambda' k' \sigma} c_{\lambda k \bar{\sigma}} | i \rangle}{(\varepsilon_\sigma - \varepsilon_{\lambda' k' \sigma})(\varepsilon_{\lambda k \bar{\sigma}} - \varepsilon_{\bar{\sigma}} - U)} \times \delta(\varepsilon_\sigma - \varepsilon_{\bar{\sigma}} - \varepsilon_{\lambda' k' \sigma} + \varepsilon_{\lambda k \bar{\sigma}}). \quad (59)$$

Note that the averaging over initial states corresponding to $|\sigma\rangle$ requires the single exchange of the operators' ordering, leading to an extra minus sign which—similarly as in the calculations of the $I_2$ part—we absorb in the denominator. Thus we obtain the same final expression as in (54).

Summing all the above contributions to the fourth order inverse lifetimes of the singly occupied level we find the following final result:

$$\gamma_\sigma^{(4)} = \frac{1}{2\pi} \sum_{\lambda,\lambda'} \int d\varepsilon [1-f_\lambda(\varepsilon)] \left[\Gamma_\sigma^\lambda \Gamma_{\bar{\sigma}}^{\lambda'} f_{\lambda'}(\varepsilon + \varepsilon_{\bar{\sigma}} - \varepsilon_\sigma) \left(\frac{(1-x)^2}{\varepsilon - \varepsilon_\sigma - U} - \frac{1}{\varepsilon - \varepsilon_\sigma}\right)^2 + f_{\lambda'}(\varepsilon) \left(\frac{\Gamma_\sigma^\lambda \Gamma_\sigma^{\lambda'}}{(\varepsilon - \varepsilon_\sigma)^2} + \frac{(1-x)^4 \Gamma_{\bar{\sigma}}^\lambda \Gamma_{\bar{\sigma}}^{\lambda'}}{(\varepsilon - \varepsilon_{\bar{\sigma}} - U)^2}\right)\right]. \quad (60)$$


[1] Ulrich Eckern, Karol I. Wysokiński, *Charge and heat transport through quantum dots with local and correlated-hopping interactions*, Phys. Rev. Research **3**, 043003 (2021).

[2] M. Lavagna, *Transport through an interacting quantum dot driven out-of-equilibrium* J. Phys. Conf. Ser. **592**, 012141 (2015).

[3] N. S. Wingreen and Y. Meir, *Anderson model out of equilibrium: Noncrossing-approximation approach to transport through a quantum dot*, Phys. Rev. B **49**, 11040 (1994).
